# Supplementary material for: Learned Sorted Table Search and Static Indexes in Small Model Space
Source: arXiv:2107.09480 source file (2022-09-17)
Supplement: Supplementary file 1 [file supp.pdf]

# Learned Sorted Table Search and Static Indexes in Small Space: Methodological and Practical Insights via an Experimental Study-Supplementary File \*

Domenico Amato<sup>1</sup>

Giosué Lo Bosco<sup>1†</sup>

Raffaele Giancarlo<sup>1</sup>

<sup>1</sup>Dipartimento di Matematica e Informatica  
Università degli studi di Palermo, ITALY  
July 21, 2021

## Abstract

This document provides additional details with respect to the content of the Main Manuscript by the same title.

## 1 Regression Analysis

It is a methodology for estimating a given function  $F : \mathbb{R}^m \rightarrow \mathbb{R}$  via a specific function model  $\tilde{F}$ . The independent variables in  $x \in \mathbb{R}^m$  and the dependent variable  $y \in \mathbb{R}$  are usually referred to as predictors and outcome, respectively. The parameters of  $\tilde{F}$  are estimated by minimizing an error function, computed using a sample set of predictors-outcome measurements.

The most commonly used Regression Loss Function is the Mean Square Error. Such a task can be accomplished in several ways. Here we follow the method outlined in [1]. In particular, we present closed-form formulae solving the posed minimization problem, as follows.

Linear Regression (**LR**, for short) is a specific approach to regression that assumes a linear function (i.e. polynomial of degree 1) as a model. The case of one predictor is referred to as Simple Linear Regression (**L**, for short), and otherwise as Multivariate Linear Regression (**M**, for short).

For **M**, given a sample set of  $n$  predictor-outcome couples  $(\mathbf{x}_i, y_i)$ , where  $\mathbf{x}_i \in \mathbb{R}^m$  and  $y_i \in \mathbb{R}$ , the goal is to characterize the linear function model  $\tilde{F}(\mathbf{x}) = \hat{\mathbf{w}}\mathbf{x}^T + \hat{b}$  by estimating the parameters  $\hat{\mathbf{w}} \in \mathbb{R}^m$  and  $\hat{b} \in \mathbb{R}$ , using the sample set. We can define a matrix  $\mathbf{Z}$  of size  $n \times (m+1)$  (usually referred to as the design matrix), where  $\mathbf{Z}_i$

is the  $i$ -th row of  $\mathbf{Z}$  such that  $\mathbf{Z}_i = [\mathbf{x}_i, 1]$ . Moreover,  $\mathbf{y}$  indicates the vector of size  $n$  such that the outcome  $y_j$  is its  $j$ -th component. The Mean Square Error minimization on the basis of the estimation is:

$$\text{MSE}(\mathbf{w}, b) = \frac{1}{n} \left\| [\mathbf{w}, b] \mathbf{Z}^T - \mathbf{y} \right\|_2^2 \quad (1)$$

**MSE** is a convex quadratic function on  $[\mathbf{w}, b]$ , so that the unique values that minimize it can be obtained by setting its gradient  $\nabla_{\mathbf{w}, b}$  equal to zero. The closed form solution for the parameters  $\mathbf{w}, b$  is

---

\*This research is funded in part by MIUR Project of National Relevance 2017WR7SHH “Multicriteria Data Structures and Algorithms: from compressed to learned indexes, and beyond”. We also acknowledge an NVIDIA Higher Education and Research Grant (donation of a Titan V GPU). Additional support to RG has been granted by Project INdAM - GNCS “Analysis and Processing of Big Data based on Graph Models”

<sup>†</sup>corresponding author, email: giosue.lobosco@unipa.it

$$[\hat{\mathbf{w}}, \hat{b}] = \mathbf{y}\mathbf{Z}(\mathbf{Z}^T\mathbf{Z})^{-1} \quad (2)$$

It is to be noted that, for  $\mathbf{L}$ , the case of models more complicated than a polynomial of degree one, specifically polynomial models with degree  $g > 1$ , can be reduced to  $\mathbf{M}$ . Indeed, we can consider the model

$$\tilde{F}(\mathbf{z}) = \sum_{i=1}^g w_i x^i + b = \mathbf{w}\mathbf{z}^T + b,$$

where  $w$  is of size  $g$ ,  $\mathbf{z} = [x, \dots, x^{g-1}, x^g] \in \mathbb{R}^g$  is the predictor vector for  $\mathbf{M}$ .

## 2 Binary, Interpolation Search and Static Learned Indexes

### 2.1 Binary Search and Its Variants

Following research in [3], with additions from [8] and with the use of the shorthand notation in the Main Text (Section 3.1), we review here two basic layouts.

- 1 Sorted. It is the classic textbook layout for standard Binary Search. In particular, we consider the branch-free implementation provided in [3], with prefetching (see Algorithm 1). The term branch-free refers to the fact that there is no branching in the while loop. Indeed, as explained in [3], the case statement in line 8 of Algorithm 1 is translated into a conditional move instruction that does not alter the flow of the assembly program corresponding to that C++ code. In turn, that has the advantage of a better use of instruction pipelining with respect to the branchy version of the same code. Prefetching, i.e., instructions 6 and 7 in Algorithm 1, refers to the fact that the procedure loads in the cache data ahead of their possible use. As shown in [3], such an implementation of Binary Search is substantially faster than its branchy counterpart. Analogous optimizations have also been considered by Shutz et al. [8]. Finally, following these latter authors, we also consider  $k$ -ary search (Algorithm 2).
- 2 Eytzinger Layout [3]. The sorted table is now seen as stored in a virtual complete balanced binary search tree. Such a tree is laid out in Breadth-First Search order in an array. An example is provided in Fig. 1. Also, in this case, we adopt a branch-free version with prefetching of the Binary Search procedure corresponding to this layout. It is reported in Algorithm 3.

---

**Algorithm 1** Branch-free implementation of classic Binary Search with prefetching. The code is as in [3] (see also [4, 8]).

---

```

1: int prefetchBranchfreeBS(int *A, int x, int left, int right){
2:   const int *base = A;
3:   int n = right;
4:   while (n > 1) {
5:     const int half = n / 2;
6:     __builtin_prefetch(base + half/2, 0, 0);
7:     __builtin_prefetch(base + half + half/2, 0, 0);
8:     base = (base[half] < x) ? &base[half] : base;
9:     n -= half;
10:  }
11:  return (*base < x) + base - A;
12: }
```

---

---

**Algorithm 2** Branch-free implementation of  $k$ -ary Binary Search, with  $k = 3$ . The code is as in [8].

---

```

    int karySearch(int *A, int x, int left, int right, int k){
2:   while (left < right) {
        int segmentLeft = left;
4:   int segmentRight = left + (right - left) / k;
        for( int i = 2; i ≤ k; ++i) {
6:       if(x ≤ A[segmentRight])
            break
8:       segmentLeft = segmentRight + 1;
        segmentRight = left + (i * (right - left)) / k;
10:    }
        left = segmentLeft;
12:    right = segmentRight;
    }
14:    return left;
    }

```

---



---

**Algorithm 3** Branch-free implementation of Binary Search with Eytzinger layout and prefetching. The code is as in [3].

---

```

    int eytzBS(int *A, int x, int left, int right){
        int i = 0;
3:   int n = right;
        while (i < n){
            __builtin_prefetch(A+(multiplier*i + offset));
6:   i = (x ≤ A[i]) ? (2*i + 1) : (2*i + 2);
        }
        int j = (i+1) >> __builtin_ffs(~(i+1));
9:   return (j == 0) ? n : j-1;
    }

```

---

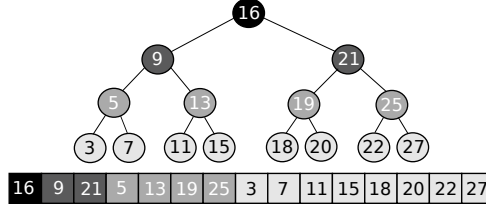

Figure 1: **An example of Eyzinger layout of a table with 15 elements.** See also [3].

## 2.2 Interpolation Search and Its Variants

As stated in the Main Text, such a Sorted Table Search technique was introduced by Peterson [7] and it has received some attention in terms of analysis [6], since it works very well on data following a Uniform or nearly Uniform distribution and very poorly on data following other distributions. The procedure adopted here is reported in

Algorithm 4. It is of interest to point out that whether a branch-free implementation of this method is advantageous with respect to its branchy version has not been extensively investigated. Experiments conducted for this study (available upon request) show that there is no advantage. As for prefetching, due to the very irregular access pattern that this procedure has to the table, it is obvious that it brings no advantage.

For completeness, we mention that modified versions of Interpolation Search have been designed, both in the static and dynamic case (see [2, 10] and references therein). Those versions can be shown to have a  $O(\log \log n)$  or even an  $O(1)$  expected time performance if the data is drawn from suitable distributions that exhibit some mathematically defined notion of regularity (see references for details). Somewhat unfortunately, those variants, although of theoretic interest, do not seem to be well suited to compete with standard Interpolation Search in real settings. In particular, the (static) variants proposed by Willard depend on three parameters  $\alpha$ ,  $\Theta$  and  $\Phi$  that are used to regularize the runtime of the procedure and that must be set through an empirical analysis. Another problem is the introduction of some arithmetic and selection operations on floating-point data types that are computationally expensive to calculate on today’s CPUs and introduce a substantial overhead in addition to element search operations.

More recently, heuristic and somewhat engineered variants of Interpolation Search have been introduced in [9].

As motivated in the Main Text, we use **TIP**, which is reported in Algorithm 5.

## 2.3 Learned Indexes

- **RMI.** It is a multi-stage model. When searching for a given key and starting with the first stage, a prediction at each stage identifies the model of the next stage to use for the next prediction. This process continues until a final stage model is reached. This latter is used to predict the interval to search into. An example is helpful.

Figure 2 describes a two-stage model. The first stage model (linear) is used to pick one of the stage 2 models (cubic). Finally, the selected model provides the final interval to search into.

- **PGM.** It is also a multi-stage model, built bottom-up and queried top down. It uses a user-defined approximation parameter  $\epsilon$ , that controls the prediction error at each stage. With reference to Figure 3, the table is subdivided into three pieces. A prediction in each piece can be done via a linear model guaranteeing an error of  $\epsilon$ . A new table is formed by selecting the minimum values in each of the three pieces. This new table is possibly again partitioned into pieces, in which a linear model can make a prediction within the given error. The process is iterated until only one linear model suffices, as in the case in the Figure. A query is processed via series of predictions, starting at the root of the tree.

- **RSI.** It is a two-stage model. It also uses user-defined approximation parameter  $\epsilon$ . With reference to Figure 4, a spline curve approximating the CDF of the data is built. Then, the radix table is used to identify spline points to use to refine the search interval. Indeed, for the key in the Figure, the most significant three bits are used to identify two spline points. Then, a binary search is performed on the table of the spline points delimited by the points identified earlier. Such a binary search identifies two spline points such that a simple interpolation guarantees a prediction with error  $\epsilon$ .

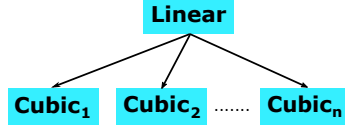

Figure 2: **An example of an RMI.** See also [5].

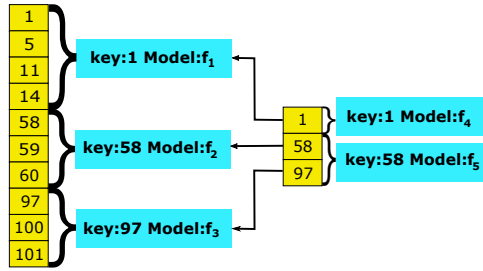

Figure 3: **An example of a PGM Index.** See also [5].

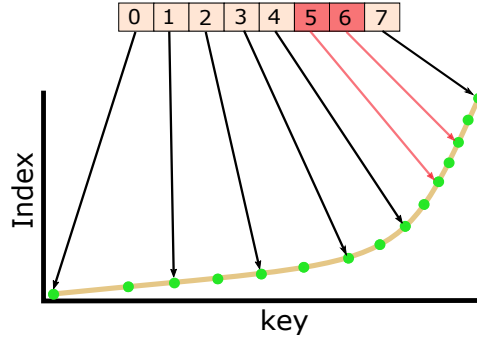

Figure 4: **An example of a RS .** See also [5].

### 3 Results of the Kolmogorov-Smirnov Test and KL Divergence Computation

With reference to the Main Text (Section 3.4), the mentioned results are reported Table 1.

---

**Algorithm 4 Implementation of Classic Interpolation Search.**

---

```
int interpolation_Search(int *arr, int x, int start, int end){
    int lo = start, hi = (end - 1);
    while (lo <= hi && x >= arr[lo] && x <= arr[hi]) {
4:     if (lo == hi) {
        if (arr[lo] == x) return lo;
        return -1;
    }
8:     int pos = lo + (((double)(hi - lo) / (arr[hi] - arr[lo])) * (x - arr[lo]));
    if (arr[pos] == x) return pos;
    if (arr[pos] < x) lo = pos + 1;
    else hi = pos - 1;
12: }
    return pos;
}
```

---

---

**Algorithm 5 TIP Interpolation Search.** The code is as in [9].

---

```
int tip(int *A, int x, int left, int right, int guard){
    int mid = end/2;
    double y0 = A[left] - x;
    double y1 = A[mid] - x;
5:  double y2 = A[right] - x;
    double num = (y1*(mid-left)*(1+(y0-y1)/(y1-y2)));
    double den = y0-y2*((y0-y1)/(y1-y2));
    int expected = mid + num / den;
    while (left < right && left <= expected &&
10:  right >= expected){
        if(abs((double)expected - (double)mid) < guard){
            return sequential(A, x, left, right);
        }
        if(A[mid] != A[expected]){
15:         left = mid;
        }else{
            right = mid;
        }
        if(expected+guard >= right || expected-guard <= left){
20:         return sequential(A, x, left, right);
        }
        mid = expected;
        y0 = A[left] - x;
        y1 = A[mid] - x;
25:     y2 = A[right] - x;
        num = (y1*(mid-right)*(mid-left)*(y2-y0));
        den = (y2*(mid-right)*(y0-y1)+y0*(mid-left)*(y1-y2));
        expected = mid + num/den;
    }
30: }
```

---

Table 1: **The results of the Kolmogorov-Smirnov Test and of the KL divergence computation.**

|               | <b>L1</b> |                   | <b>L2</b> |                    | <b>L3</b> |                    |
|---------------|-----------|-------------------|-----------|--------------------|-----------|--------------------|
| Datasets      | %succ     | KLdiv             | %succ     | KLdiv              | %succ     | KLdiv              |
| <b>amzn32</b> | 100       | 1.87e-05±1.41e-13 | 100       | 1.58e-04 ±8.76e-13 | 100       | 3.77e-03 ±2.20e-11 |
| <b>amzn64</b> | 100       | 9.54e-06±7.27e-14 | 100       | 7.88e-05±7.97e-13  | 100       | 1.88e-03±1.52e-11  |
| <b>face</b>   | 100       | 1.98e-05±1.00e-12 | 100       | 7.98e-05±4.43e-13  | 100       | 1.88e-03±1.24e-11  |
| <b>osm</b>    | 100       | 9.38e-06±4.51e-14 | 100       | 7.88e-05±3.46e-13  | 100       | 1.88e-03±9.55e-12  |
| <b>wiki</b>   | 100       | 9.47e-06±5.27e-14 | 100       | 7.87e-05±5.64e-13  | 100       | 1.88e-03±1.25e-11  |

Table 2: **Training time for L1 tables, in seconds and per element.** The first column indicated the datasets. The remaining columns indicate the model used for the learning phase. Abbreviations are as in the main text. The **SOSD** columns refer to the entire output of that library, averaged over a number of models and elements in each table.

|               | <b>L</b>             | <b>Q</b> | <b>C</b> | <b>15O-BFS</b> | <b>SY-RMI 2%</b> | <b>SOSD RMI</b> | <b>SOSD RS</b> | <b>SOSD PGM</b> |
|---------------|----------------------|----------|----------|----------------|------------------|-----------------|----------------|-----------------|
| Datasets      | <b>Training Time</b> |          |          |                |                  |                 |                |                 |
| <b>amzn32</b> | 6.2e-07              | 4.3e-08  | 5.7e-08  | 8.0e-07        | 3.5e-06          | 1.2e-06         | 1.8e-06        | 5.4e-08         |
| <b>amzn64</b> | 7.3e-08              | 8.7e-08  | 1.0e-07  | 5.3e-07        | 2.6e-07          | 3.6e-07         | 2.8e-06        | 6.2e-08         |
| <b>face</b>   | 3.0e-07              | 7.7e-08  | 8.5e-08  | 5.5e-07        | 7.5e-06          | 6.7e-07         | 8.2e-07        | 5.7e-08         |
| <b>osm</b>    | 6.9e-08              | 7.4e-08  | 9.9e-08  | 4.6e-07        | 4e-05            | 4.6e-06         | 5.5e-06        | 5.0e-08         |
| <b>wiki</b>   | 6.8e-08              | 1.4e-07  | 7.9e-08  | 9.0e-07        | 6.9e-06          | 3.7e-07         | 8.7e-06        | 4.6e-08         |

For each memory level (first row) and each original dataset (first column), it is reported the percentage of times in which the Kolmogorov-Smirnov test failed to report a difference between the CDFs of the dataset extracted uniformly and at random from the original one and this latter, over 100 extractions. Moreover, the KL divergence between the PDFs of the chosen generated dataset and the original one is also reported.

## 4 Learning the CDF of a Sorted Table: Full Set of Experiments

Tables 2-5 report the full set of experiments described and discussed in Section ?? of the Main Text.

## 5 Constant Space Models: Full Set of Query Experiments

Figures 5-10 report the full set of experiments described and discussed in Section 5 of the Main Text.

Table 3: **Training time for L2 tables, in seconds and per element.** The table legend is as in Table 2

|               | <b>L</b>             | <b>Q</b> | <b>C</b> | <b>15O-BFS</b> | <b>SY-RMI 2%</b> | <b>SOSD RMI</b> | <b>SOSD RS</b> | <b>SOSD PGM</b> |
|---------------|----------------------|----------|----------|----------------|------------------|-----------------|----------------|-----------------|
| Datasets      | <b>Training Time</b> |          |          |                |                  |                 |                |                 |
| <b>amzn32</b> | 1.0e-08              | 7.7e-08  | 1.4e-07  | 1.1e-07        | 5.6e-06          | 4.6e-07         | 2.3e-07        | 4.2e-08         |
| <b>amzn64</b> | 1.6e-08              | 2.7e-07  | 3.1e-07  | 1.8e-07        | 5.2e-06          | 5.6e-07         | 3.5e-07        | 5.0e-08         |
| <b>face</b>   | 1.4e-08              | 2.7e-07  | 2.8e-07  | 1.0e-07        | 4.1e-06          | 4.6e-07         | 1.1e-07        | 3.9e-08         |
| <b>osm</b>    | 1.3e-08              | 2.7e-07  | 2.9e-07  | 1.2e-07        | 2.8e-04          | 2.9e-05         | 6.9e-07        | 4.0e-08         |
| <b>wiki</b>   | 1.7e-08              | 2.7e-07  | 2.7e-07  | 1.0e-07        | 7.8e-06          | 9.3e-07         | 1.0e-06        | 3.7e-08         |

Table 4: **Training time for L3 tables, in seconds and per element.** The table legend is as in Table 2

|               | <b>L</b>             | <b>Q</b> | <b>C</b> | <b>15O-BFS</b> | <b>SY-RMI 2%</b> | <b>SOSD RMI</b> | <b>SOSD RS</b> | <b>SOSD PGM</b> |
|---------------|----------------------|----------|----------|----------------|------------------|-----------------|----------------|-----------------|
| Datasets      | <b>Training Time</b> |          |          |                |                  |                 |                |                 |
| <b>amzn32</b> | 1.1e-08              | 1.7e-08  | 2.3e-08  | 5.3e-08        | 4.5e-06          | 5.0e-07         | 1.7e-08        | 2.7e-08         |
| <b>amzn64</b> | 1.6e-08              | 2.0e-08  | 1.9e-08  | 6.3e-08        | 1.5e-06          | 1.3e-07         | 2.4e-08        | 3.4e-08         |
| <b>face</b>   | 8.2e-09              | 2.1e-08  | 1.9e-08  | 3.9e-08        | 1.5e-05          | 1.6e-06         | 1.4e-08        | 2.4e-08         |
| <b>osm</b>    | 1.6e-08              | 1.9e-08  | 2.0e-08  | 4.4e-08        | 1.2e-05          | 1.3e-06         | 3.5e-08        | 3.8e-08         |
| <b>wiki</b>   | 1.5e-08              | 2.0e-08  | 1.9e-08  | 4.1e-08        | 2.3e-06          | 2.2e-07         | 5.1e-08        | 3.7e-08         |

Table 5: **Training time for L4 tables, in seconds and per element.** The table legend is as in Table 2

|               | <b>L</b>             | <b>Q</b> | <b>C</b> | <b>15O-BFS</b> | <b>SY-RMI 2%</b> | <b>SOSD RMI</b> | <b>SOSD RS</b> | <b>SOSD PGM</b> |
|---------------|----------------------|----------|----------|----------------|------------------|-----------------|----------------|-----------------|
| Datasets      | <b>Training Time</b> |          |          |                |                  |                 |                |                 |
| <b>amzn32</b> | 7.9e-09              | 1.4e-08  | 1.4e-08  | 3.7e-08        | 1.2e-06          | 1.2e-07         | 9.5e-09        | 2.4e-08         |
| <b>amzn64</b> | 7.9e-09              | 1.4e-08  | 1.4e-08  | 3.7e-08        | 1.1e-06          | 2.2e-07         | 2.1e-08        | 5.0e-08         |
| <b>face</b>   | 8.0e-09              | 1.4e-08  | 1.4e-08  | 3.6e-08        | 1.3e-06          | 2.5e-07         | 2.1e-08        | 6.5e-08         |
| <b>osm</b>    | 8.0e-09              | 1.4e-08  | 1.4e-08  | 3.6e-08        | 1.2e-06          | 2.5e-07         | 2.2e-08        | 7.4e-08         |
| <b>wiki</b>   | 7.9e-09              | 1.4e-08  | 1.4e-08  | 3.6e-08        | 1.1e-06          | 2.2e-07         | 1.9e-08        | 4.1e-08         |

## 6 Parametric Space Models:Query Experiments

Figures 11-15 report the full set of experiments described and discussed in 6 of the Main Text.

## References

- [1] Ian Goodfellow, Yoshua Bengio, and Aaron Courville. *Deep Learning*. The MIT Press, 2016.
- [2] Alexis Kaporis, Christos Makris, Spyros Sioutas, Athanasios Tsakalidis, Kostas Tsihlias, and Christos Zaroliagis. Dynamic interpolation search revisited. pages 382–394, 07 2006.
- [3] Paul-Virak Khuong and Pat Morin. Array Layouts for Comparison-Based Searching. *J. Exp. Algorithms*, 22:1.3:1–1.3:39, 2017.
- [4] Donald E. Knuth. The Art of Computer Programming, vol. 3 (sorting and searching). *Addison-Wesley Publishing Company*, 3:481–489, 1973.
- [5] Ryan Marcus, Andreas Kipf, Alexander van Renen, Mihail Stoian, Sanchit Misra, Alfons Kemper, Thomas Neumann, and Tim Kraska. Benchmarking learned indexes. 14:1–13, 2020.
- [6] K. Mehlhorn and A. Tsakalidis. Data Structures. In *Handbook of Theoretical Computer Science (Vol. A): Algorithms and Complexity*, page 302–341. MIT Press, Cambridge, MA, USA, 1991.
- [7] W. W. Peterson. Addressing for random-access storage. *IBM Journal of Research and Development*, 1(2):130–146, 1957.
- [8] Lars-Christian Schulz, David Broneske, and Gunter Saake. An eight-dimensional systematic evaluation of optimized search algorithms on modern processors. *Proc. VLDB Endow.*, 11:1550–1562, 2018.
- [9] Peter Van Sandt, Yannis Chronis, and Jignesh M. Patel. Efficiently Searching In-Memory Sorted Arrays: Revenge of the Interpolation Search? In *Proceedings of the 2019 International Conference on Management of Data, SIGMOD ’19*, pages 36–53, New York, NY, USA, 2019. ACM.

- [10] D. E. Willard. Searching unindexed and nonuniformly generated files in  $\log\log N$  time. *SIAM J Comput.* Vol. 14, pages 1013–1029, 1985.

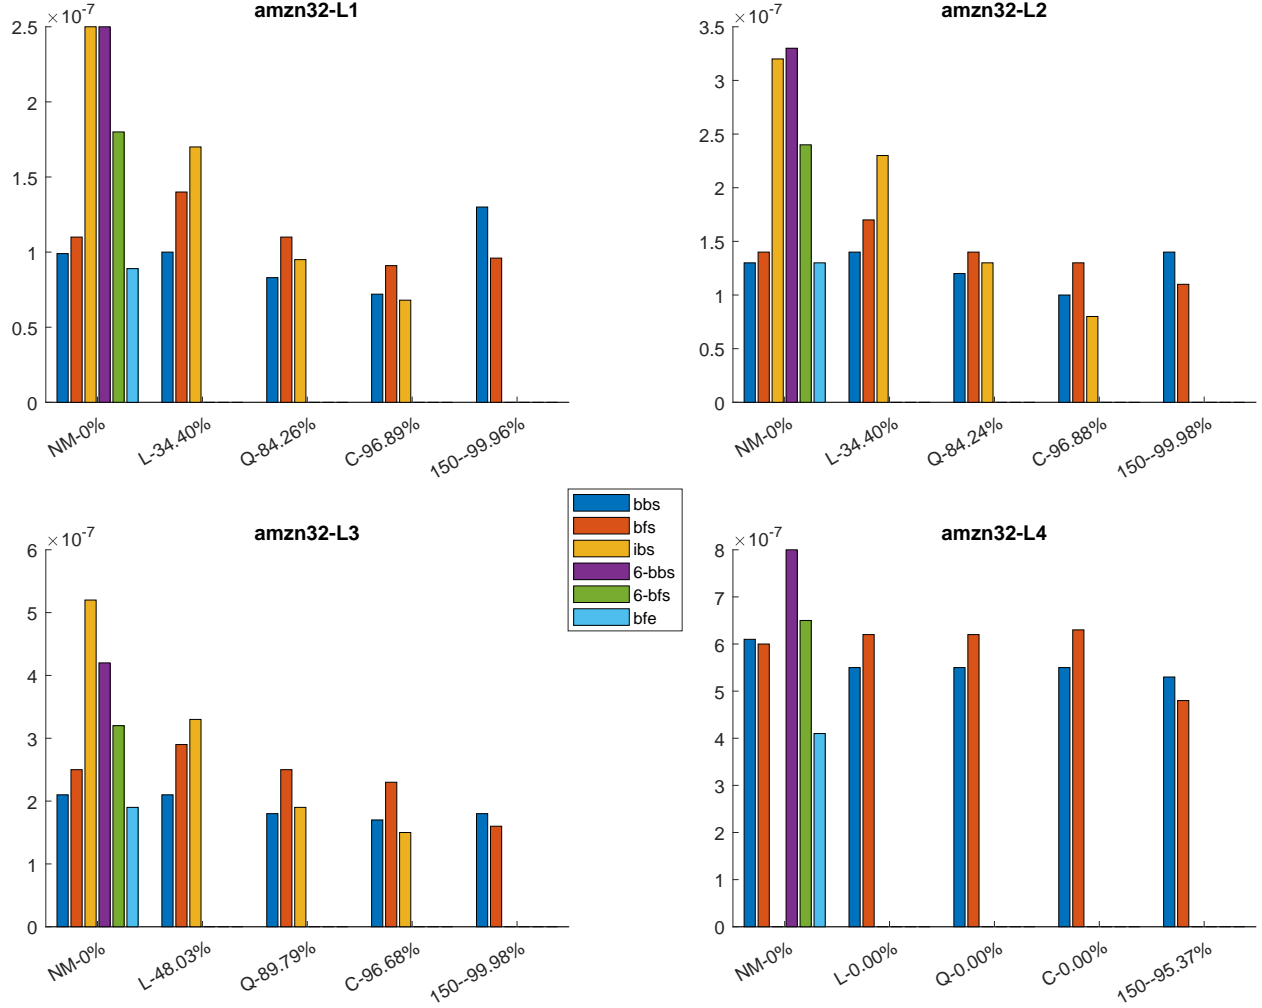

Figure 5: **Query times for the amzn32 dataset on Sorted Table Search Procedures.** The methods are the ones in the legend (middle of the four panels, the notation is as in main text and each method has a distinct color). For each memory level, the abscissa reports methods grouped by model. From left to right, no model, linear, quadratic, cubic and **KO-**, with  $k = 15$ , and with **BFS** and **BBS** as search methods. **K-BFS** is reported with  $k = 6$ . For those latter, the reduction factor corresponding to the table is also reported. On the ordinate, it is reported the average query time, in seconds. For memory levels **L4**, **IBS**, **L-IBS**, **Q-IBS** and **C-IBS** have been excluded, since inclusion of their query time values ( $1.4e-05$ ,  $1.6e-05$ ,  $1.6e-05$ ,  $1.4e-05$ , respectively) would make the histograms poorly legible.

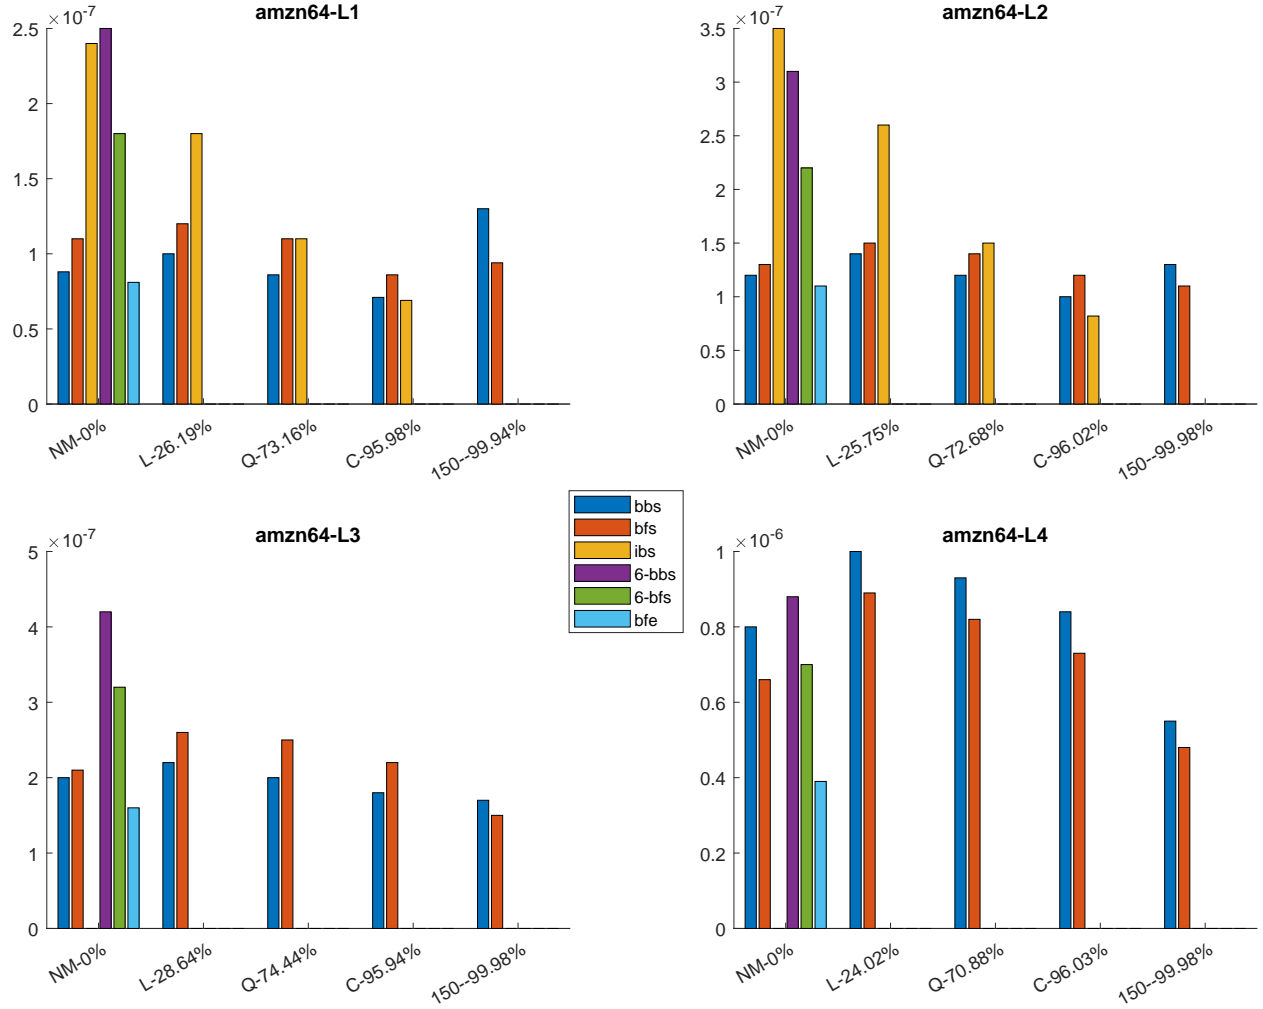

Figure 6: **Query times for the amzn64 dataset on Sorted Table Search Procedures.** The figure legend is as in Figure 5. For memory level **L4**, **IBS**, **L-IBS** and **Q-IBS** have been excluded, since inclusion of their query time values ( $3.1\text{e-}06$ ,  $2.1\text{e-}06$ ,  $1.2\text{e-}06$ , respectively) would make the histograms poorly legible.

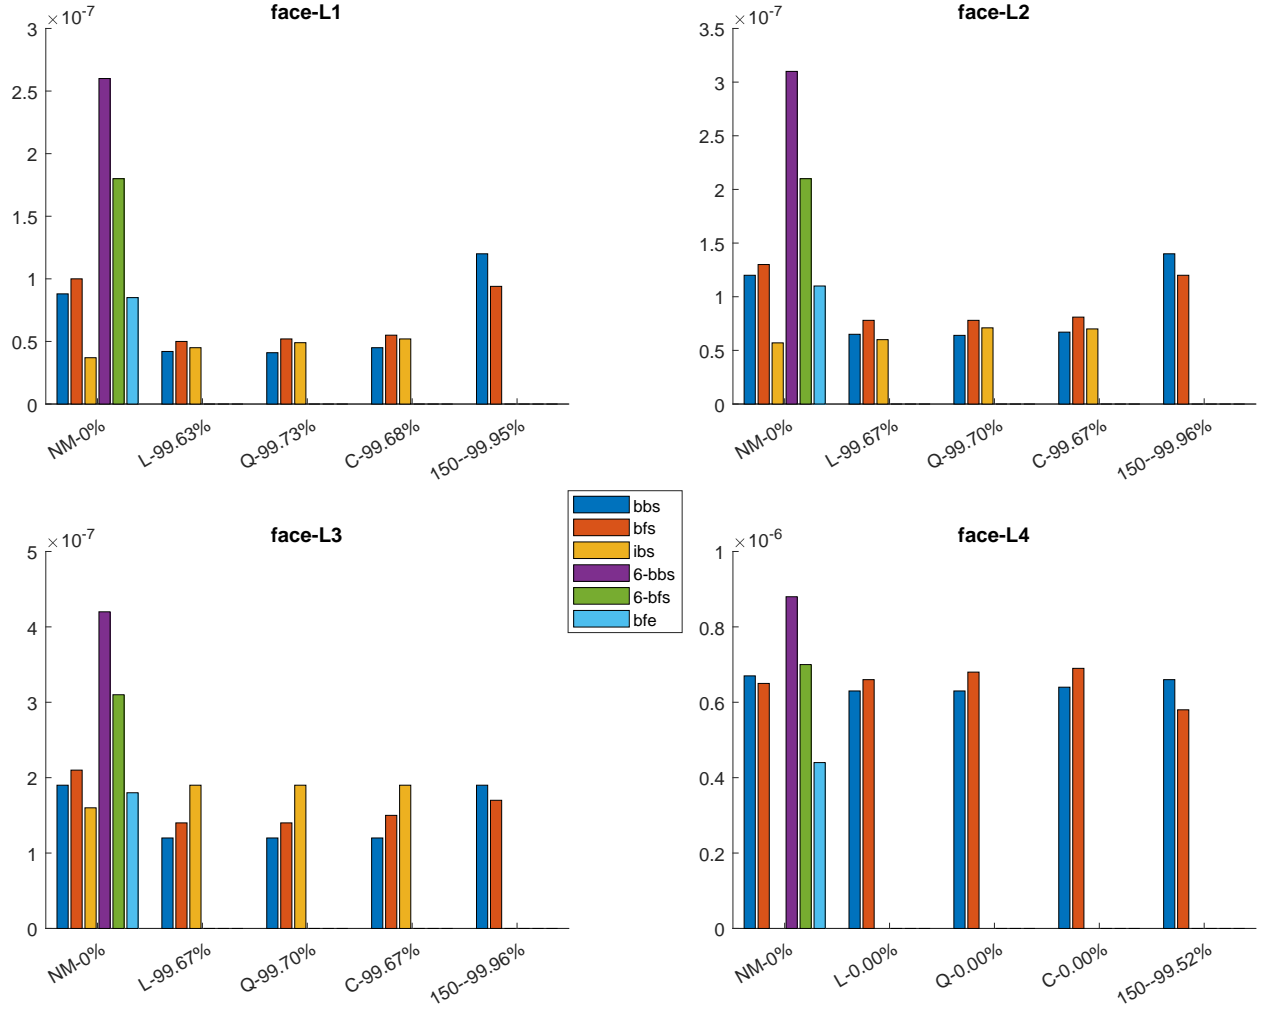

Figure 7: **Query times for the face dataset on Sorted Table Search Procedures.** The figure legend is as in Figure 5. For memory levels **L4**, **IBS** and its Learned versions have been excluded because of their poor performance (data not shown and available upon request).

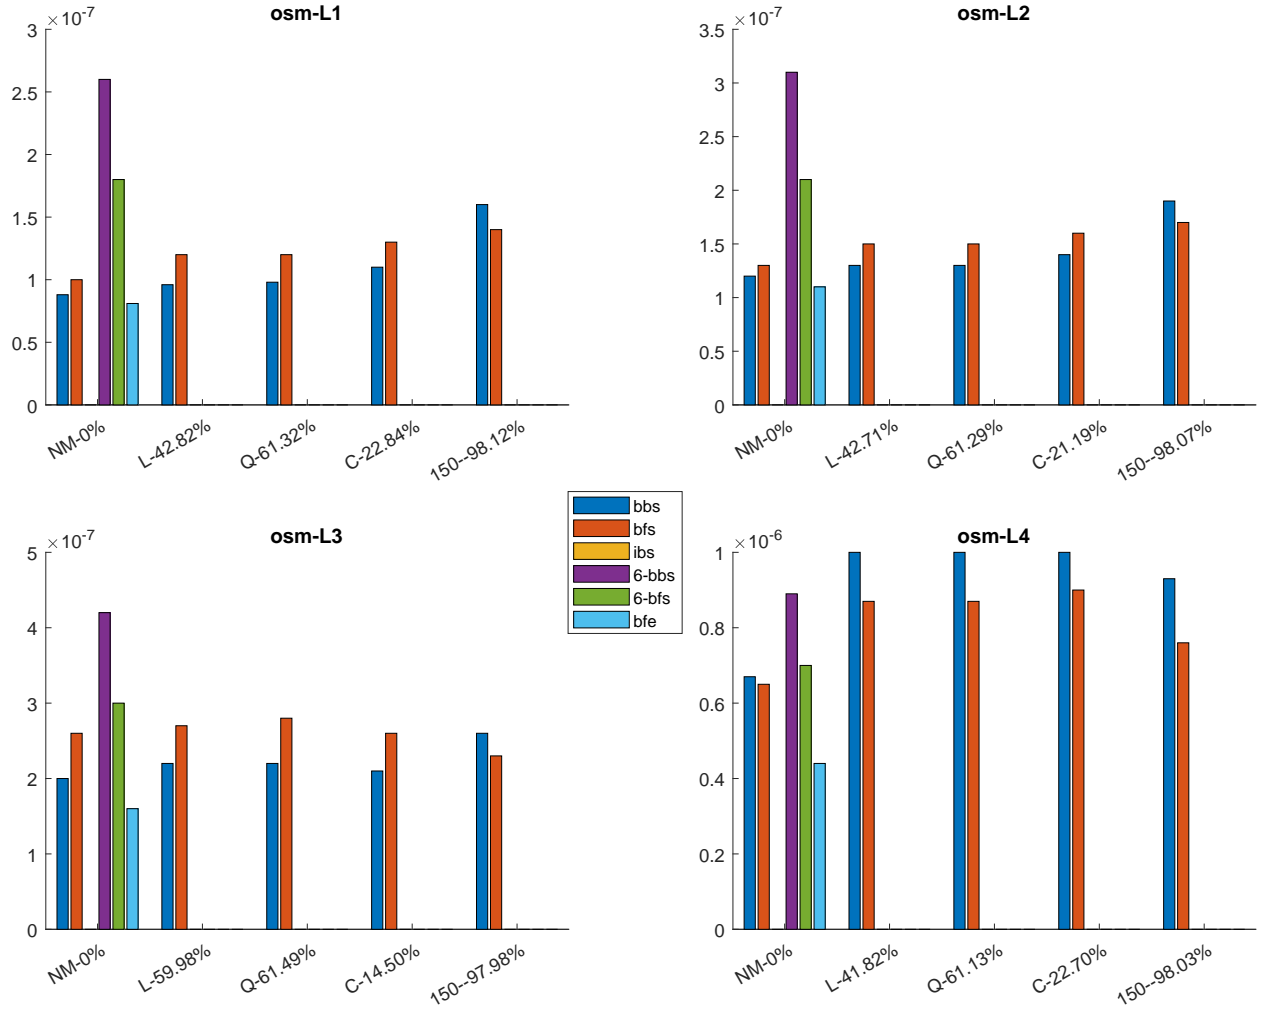

Figure 8: **Query times for the osm dataset on Sorted Table Search Procedures.** The figure legend is as in Figure 5. For all memory levels, **IBS** has been excluded, since inclusion of its query time values ( $1.2e-06$ ,  $2.2e-06$ ,  $6.5e-06$ ,  $6.4e-05$ , respectively) would make the histograms poorly legible. Its regression-based Learned versions have been excluded for the same reason (data not shown and available upon request). However, they have better query time performance with respect to **IBS**, in particular **Q** and **C**.

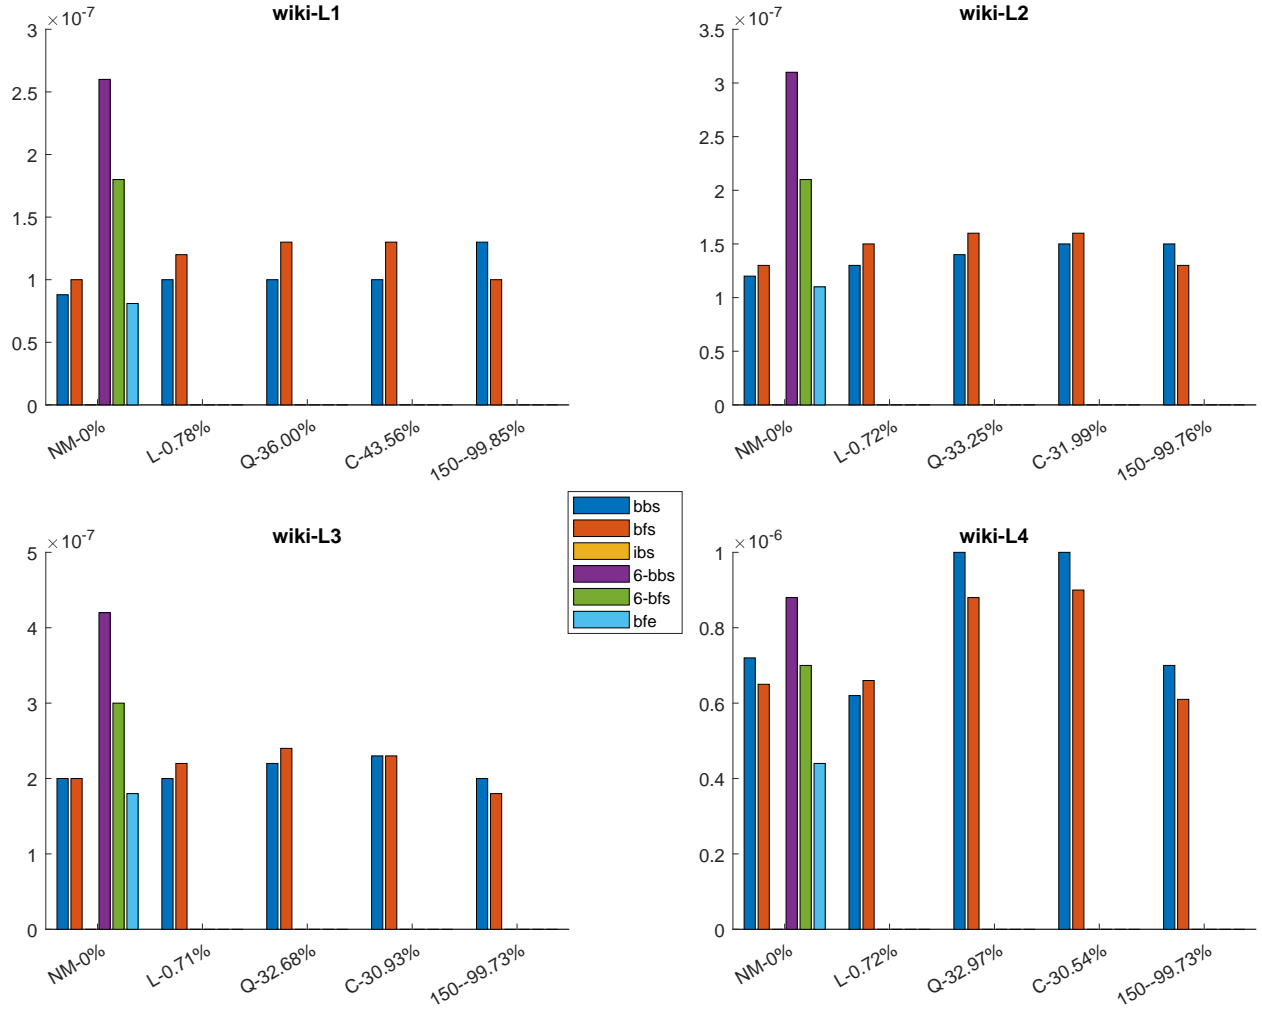

Figure 9: **Query times for the wiki dataset on Sorted Table Search Procedures.** The figure legend is as in Figure 5. For all memory levels, **IBS** has been excluded, since inclusion of its query time values ( $3.1\text{e-}07$ ,  $5.1\text{e-}07$ ,  $9.5\text{e-}07$ ,  $5.1\text{e-}06$ , respectively) would make the histograms poorly legible. Its regression-based Learned versions have been excluded for the same reason (data not shown and available upon request). However, they have better query time performance with respect to **IBS**, in particular **Q** and **C**.

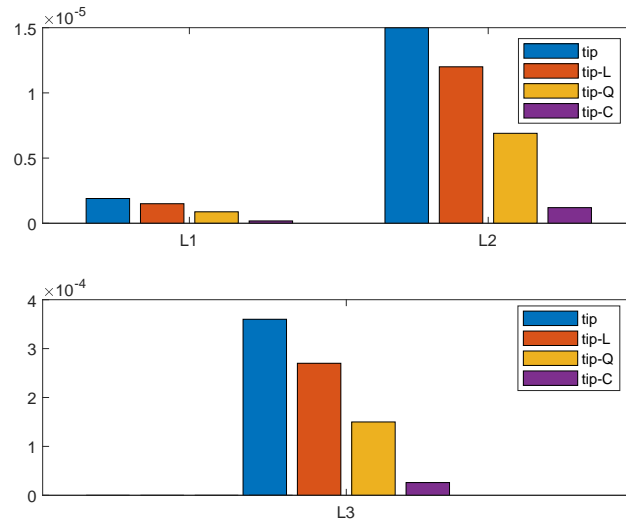

Figure 10: **Query times for TIP and its Learned Variants on the amzn32 dataset**, for the first three memory levels. On the fourth, the procedures were stopped due to their poor execution times. The figure legend is as in Figure 5.

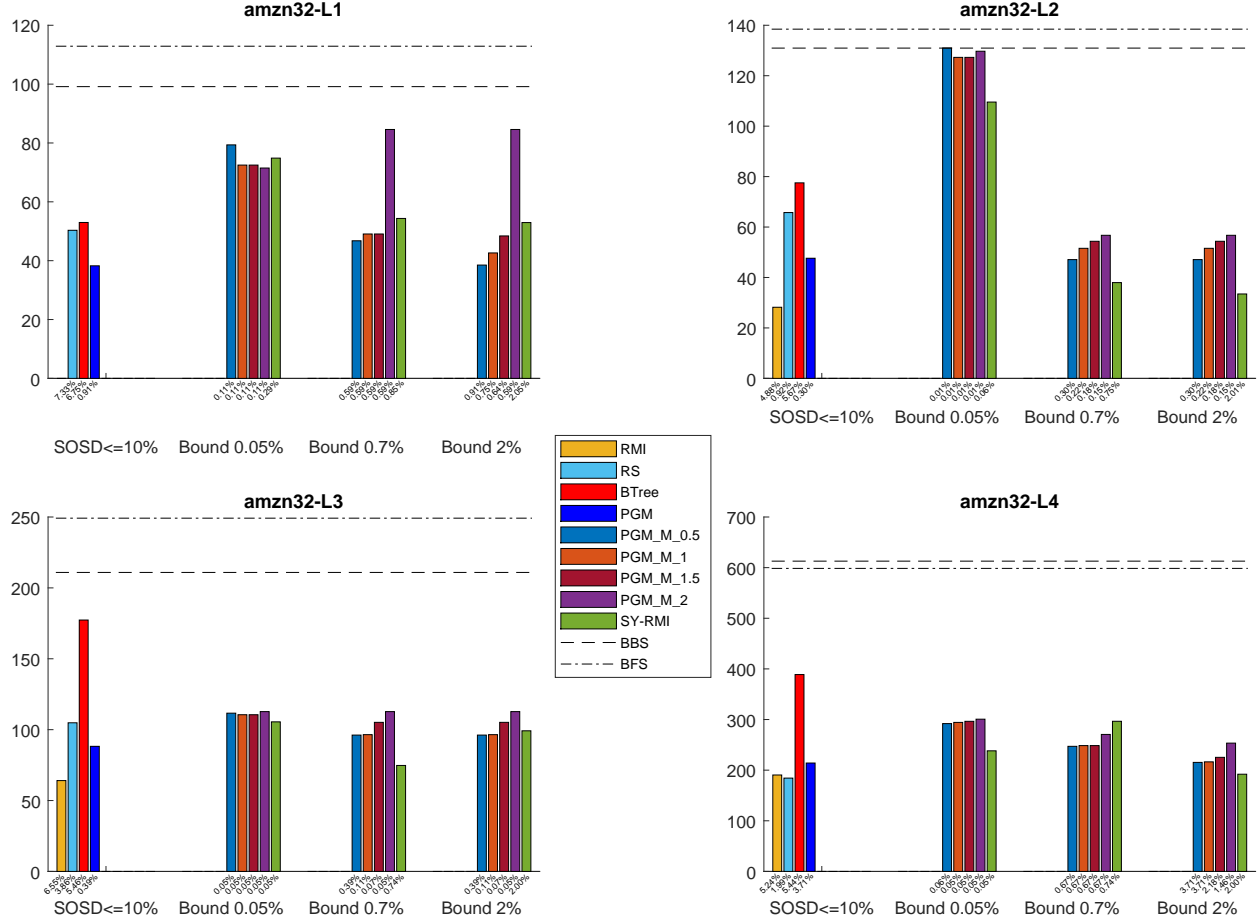

Figure 11: **Query times for the amzn32 dataset on Learned Indexes in Small Space.** The methods are the ones in the legend (middle of the four panels, the notation is as in the main text and each method has a distinct color). For each memory level, the abscissa reports methods grouped by space occupancy, as specified in the main text. When no model in a class output by **SOSD** takes at most 10% of additional space, that class is absent. The ordinate reports the average query time, with **BBS** and **BFS** executed in **SOSD** as baseline (horizontal lines).

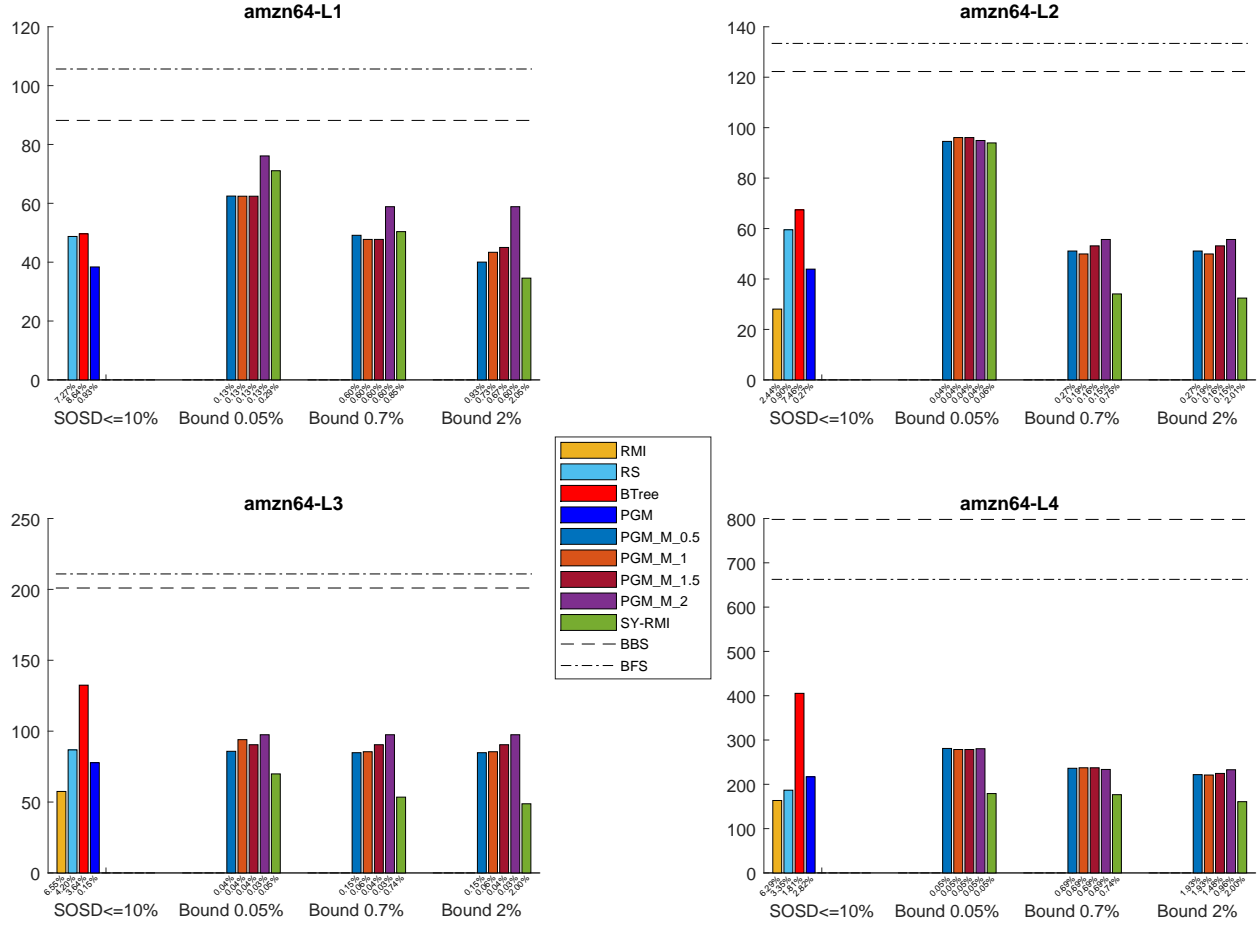

Figure 12: Query times for the amzn64 dataset on Learned Indexes in Small Space. The figure legend is as in Figure 11.

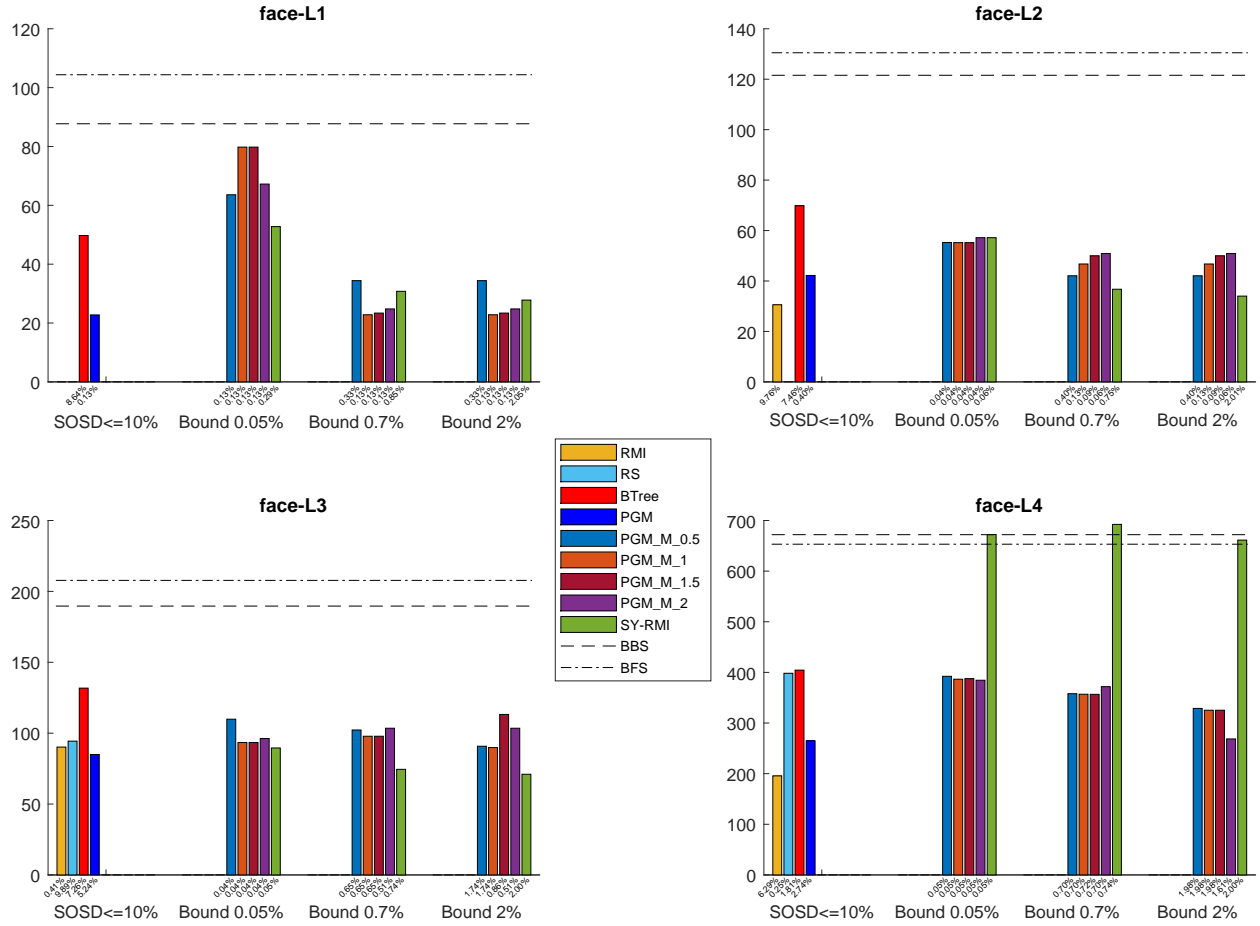

Figure 13: Query times for the face dataset on Learned Indexes in Small Space. The figure legend is as in Figure 11.

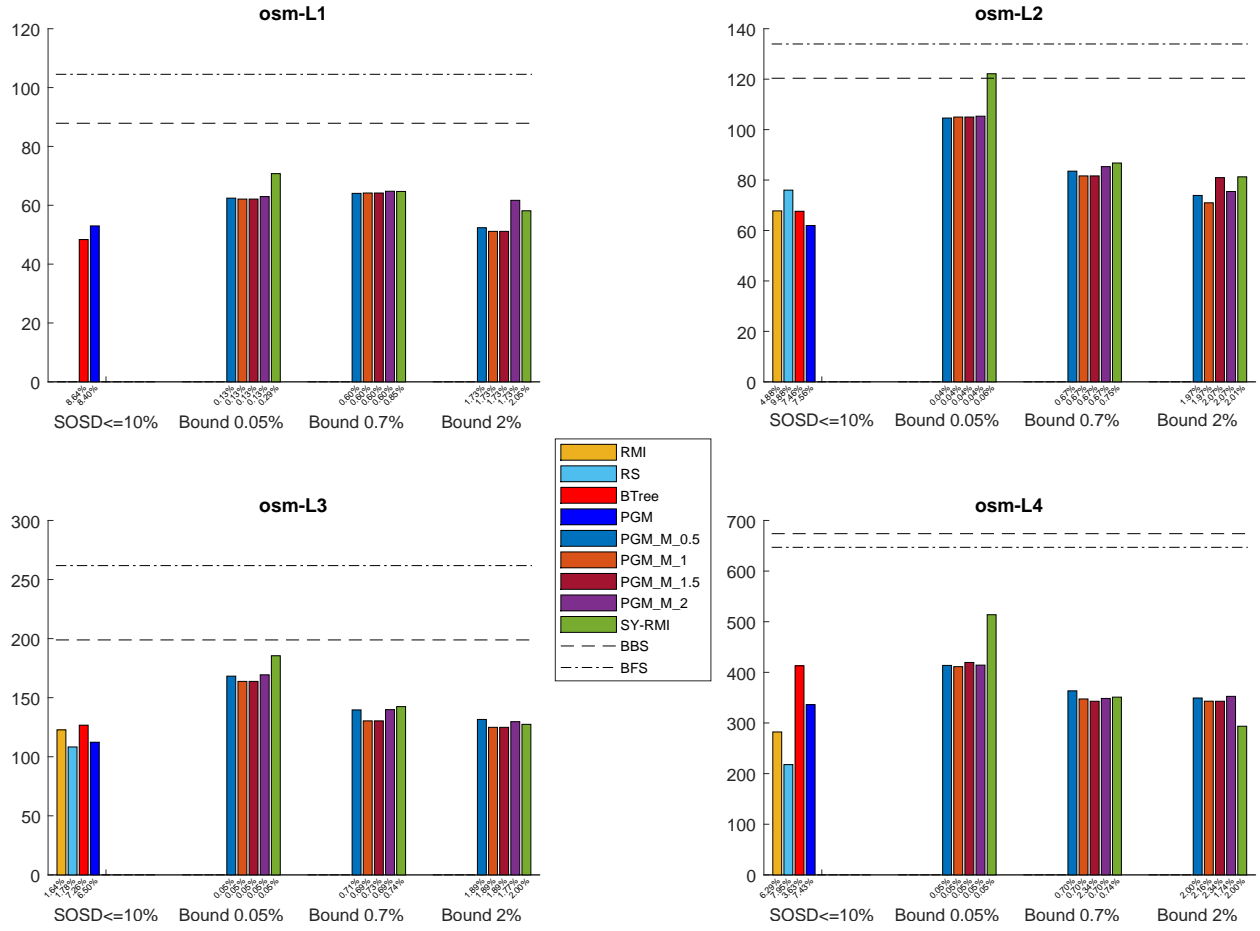

Figure 14: Query times for the osm dataset on Learned Indexes in Small Space. The figure legend is as in Figure 11.

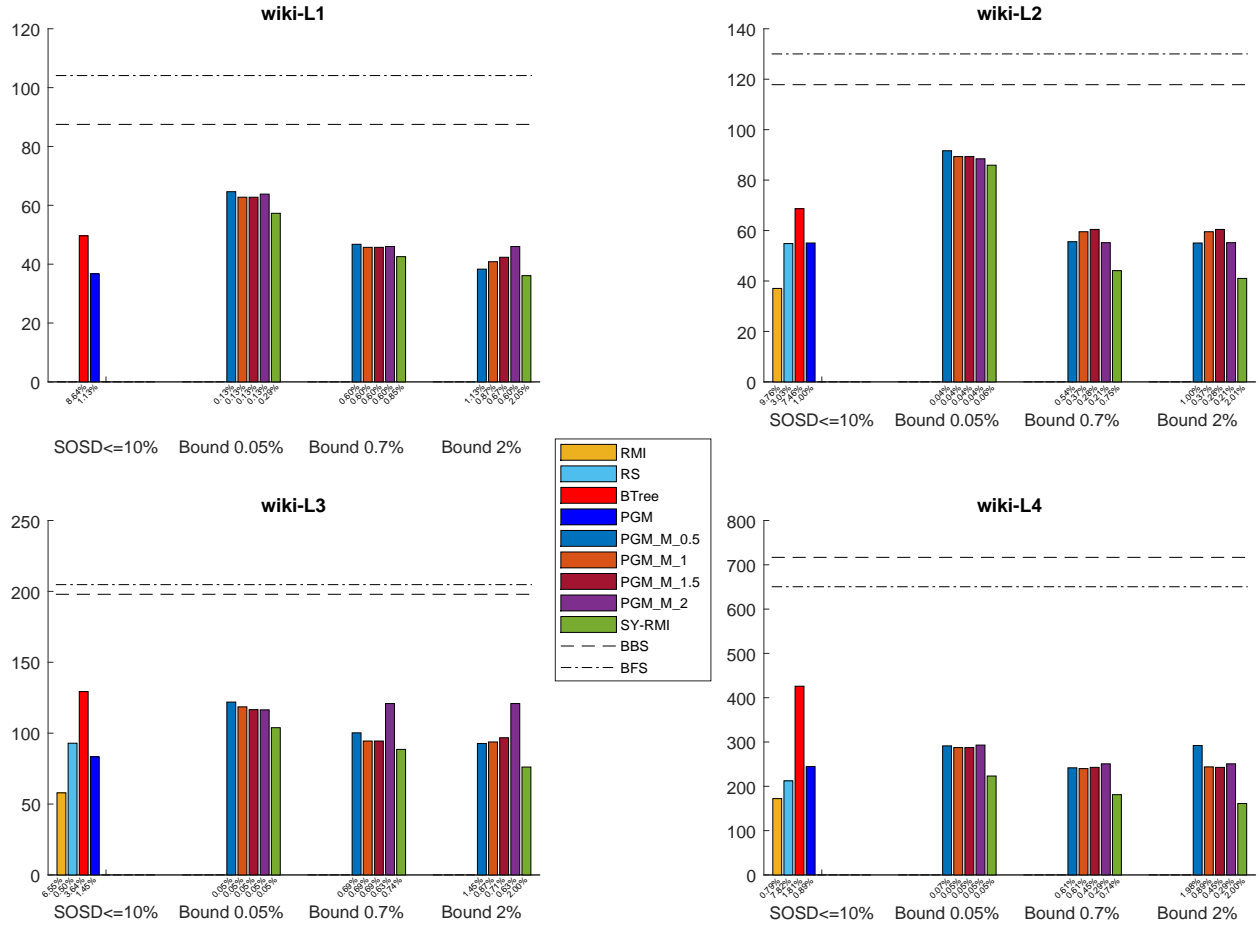

Figure 15: Query times for the wiki dataset on Learned Indexes in Small Space. The figure legend is as in Figure 11.
